# Supplementary material for: Tug-of-War: Observations on Unified Content Handling
Source: arXiv:1708.09334 source file (2017-08-29)
Supplement: Supplementary file 1 [file appendix.tex]

\appendix

\subsection{Lifecycle of Web Content Handling}

To investigate the possible discrepancies in handling of web content on a
system, we delineate the lifecycle stages from when the web content is
first served from the web server to when the web content is handled on the
system. This facilitates a systematic exploration of the different stages
to uncover possible discrepancies in the way the content is handled across
disparate components on a system.

\subsection{Content Handling by the OS}
\label{subsec:os_mime}

\subsubsection{Linux}
\label{subsubsec:os_ub}

In Linux, the mapping between file extensions and MIME types is stored in
\texttt{/etc/mime.types}. If a file has an extension the OS will open it with
the default application for the corresponding MIME type. Each application
registers the MIME types it can handle in a dedicated \textit{Desktop Entry
Specification} (\texttt{.desktop}), usually located under
(\texttt{/usr/share/applications}). User entries are stored under \textit{
    \$HOME/.local/share/applications}~\footnote{note that the exact path varies
based on the distribution and the desktop manager, for isntance could be
\texttt{~/.gnome2/vfolders/applications} for Fedora-Gnome \etc} and take
precedence over System entries. Active application schemas can be listed with
\texttt{gsettings list-schemas}. In case a user wants to have \texttt{.desktop}
files at other locations, they need to be executable, so as to avoid
accidentally running arbitrary code from files downloaded from the
Internet~\cite{desktop_linux:online}~\footnote{\#!/usr/bin/xdg-open can be used
at the beginning of the file to make it a valid executable script which will
launch the application when executed}

Additional notes:
\begin{itemize}
    \item {\texttt{desktop-file-install} installs \texttt{.desktop} files to the
        user's applications directory when run as a non-root user, and to
        \texttt{/usr/share/applications} if run as root}
    \item {\texttt{update-desktop-database} and \texttt{update-mime-database}
        update the \texttt{.desktop} entries and MIME type databases
        respectively}
    \item { An alternate way to add a MIME type except for editiing
        \texttt{/etc/mime.types} is to register an XML documents in the
        \texttt{/usr/share/mime/} directory, followed by a
        \texttt{update-mime-database /usr/share/mime} call.
        \theo{Q1: will this be read at start-up if no update command is run?
        Q2:Does this command append to /etc/mime.types?}}
    \item {We can get the default application that handles files of a particular
        MIME type by running \\ \texttt{xdg-mime query default <MIME>}}
    \item {We can set the default application to handles files of a particular
        MIME type by running \\ \texttt{xdg-mime default <APP> <MIME>}}
\end{itemize}

In case of an extensionless file, the OS attempts to do MIME-type sniffing
based on magic values that might be present. The information regarding these
files is read from \texttt{/etc/magic} and the compiled magic file
\texttt{/usr/share/misc/magic.mgc}, or the files in the directory
\texttt{/usr/share/misc/magic} if the compiled file does not exist.  If a file
does not match any of the entries in the magic file, it is examined to see if it
seems to be a text file.

\theo{URL Handler info}

\subsubsection{Mac OS X}
\label{subsubsec:os_osx}
\textbf{LaunchServices}:
Active LaunchServices URL handler settings can be read via

\texttt{\tiny{defaults read
com.apple.LaunchServices/com.apple.launchservices.secure}}

The lsregister command is actually just a front-end management tool for the
\texttt{\tiny{~/Library/Preferences/com.apple.LaunchServices.plist}} file. The
file's
contents can be read (in an unparsed form) using defaults:

\texttt{\tiny{defaults read ~/Library/Preferences/com.apple.LaunchServices}}

\subsubsection{Windows}
\label{subsubsec:os_win}
Windows opens files based on their extension. Each mime type and extension
association is contained in
\textit{HKEY\_CLASSES\_ROOT$\backslash$MIME$\backslash$Database$\backslash$Content}

\subsubsection{Android}
\label{subsubsec:os_android}

\subsubsection{iOS}
\label{subsubsec:os_ios}

\subsection{Browser MIME-Type Handling}
\label{subsec:back_content_handling}
In order to shed light on the different behaviors that browsers exhibit when
handling content, we analyze popular browsers currently in use, namely
Google's Chrome, Microsoft's Internet Explorer and Edge,
Mozilla's Firefox, Apple's Safari as well as the Opera browser. Overall, these
browsers cover more than than XX\% percent of the market
~\cite{browser_stats_w3c,browser_stats_dgov}

\subsubsection{Noteworthy Quirks}
\begin{itemize}

\item Pepper Plugin API (PPAPI) is a browser plug-in model extension that
enables out-of-process plug-in execution~\cite{ppapi:online}. Pepper is
supported by Chrome, and Blink layout engine-based browsers such as Opera.
For example, in Opera, there is whitelist of MIME types
(\texttt{application/x-ppapi-widevine-cdm} and
\texttt{application/x-google-chrome-pdf}), which when encountered
will invoke specific PPAPI processes (\texttt{widevinecdmadapter.plugin} and
\texttt{Chrome internal-pdf-viewer} respectively). Any potential for vulnerabilities?

\end{itemize}

\subsubsection{Browser: Chrome}
\label{subsubsec:chrome_mime_handling}

\subsubsection{Browser: Firefox}
\label{subsubsec:firefox_mime_handling}

%node distance
\newdimen\ndist
\ndist=3cm
\tikzstyle{level 1}=[level distance=\ndist, sibling distance=\ndist]
\tikzstyle{level 2}=[level distance=\ndist, sibling distance=\ndist]

% Define styles for qs and leafs
\tikzstyle{q} = [text width=8em, text justified]
\tikzstyle{end} = [circle, minimum width=3pt,fill, inner sep=0pt]

% The sloped option gives rotated edge labels. Personally
% I find sloped labels a bit difficult to read. Remove the sloped options
% to get horizontal labels.
\begin{figure*}[th!]
\begin{tikzpicture}[grow=right, sloped]
\node[q] {Auto-download?}
    [clockwise from=85]
    child [level distance=8em, sibling angle=0] {
        node[q] {Is MIME type set?}
            [clockwise from=20]
            child [level distance=8em, sibling angle=0]
            {
                node[q]
                {Does the MIME type agree with the extension?}
                    [clockwise from=10]
                    child [level distance=8em, sibling angle=0]
                    {
                        node[end, label=right: {
                            Prompt with notice of the document type
                        (e.g. ``PDF", ``ZIP")\theo{638.350.350}}] {}
                        edge from parent
                        node[above] {$yes$}
                    }
                    child [level distance=8em, sibling angle=10]
                    {
                        node[end, label=right:
                        {Promt showing MIME type}] {}
                        edge from parent
                        node[above] {$no$}
                    }
                edge from parent
                node[above] {$yes$}
            }
            child [level distance=8em, sibling angle=50]
            {
                node[q] {Can we sniff?}
                    [clockwise from=20]
                    child [level distance=8em, sibling angle=0]
                    {
                        node[q]
                        { Does payload match extension? }
                            [clockwise from=10]
                            child [level distance=8em, sibling angle=0]
                            {
                                node[end, label=right: {
                                    Prompt with notice of the document type
                                (e.g. ``PDF")\theo{350.642.350}}] {}
                                edge from parent
                                node[above] {$yes$}
                            }
                            child [level distance=8em, sibling angle=15]
                            {
                                node[end, label=right:
                                {Promt showing MIME type\theo{350.642.638}}] {}
                                node[above] {$no$}
                            }
                        edge from parent
                        node[above] {$yes$}
                    }
                    child [level distance=8em, sibling angle=40]
                    {
                        node[q]
                        {Is auto-open set? }
                            [clockwise from=10]
                            child [level distance=8em, sibling angle=0]
                            {
                                node[end, label=right: {
                                    Open with speficied program}] {}
                                edge from parent
                                node[above] {$yes$}
                            }
                            child [level distance=8em, sibling angle=10]
                            {
                                node[end, label=right:
                                {Download\theo{634.642.638}}] {}
                                edge from parent
                                node[above] {$no$}
                            }
                        edge from parent
                        node[above] {$no$}
                    }
                edge from parent
                node[above] {$no$}
            }
            edge from parent
            node[above] {$yes$}
    }
    child [level distance=8em, sibling angle=165] {
        node[q] {Is MIME type set?}
            [clockwise from=20]
            child [level distance=8em, sibling angle=0]
            {
                node[q]
                {Can it be rendered based on MIME type?}
                    [clockwise from=10]
                    child [level distance=8em, sibling angle=0]
                    {
                        node[end, label=right: {
                            Render as denoted by MIME
                        }] {}
                        edge from parent
                        node[above] {$yes$}
                    }
                    child [level distance=8em, sibling angle=30]
                    {
                        node[q]
                        {Is auto-open set? }
                            [clockwise from=10]
                            child [level distance=8em, sibling angle=0]
                            {
                                node[end, label=right: {
                                    Open with speficied
                                    program~\theo{350.642.642}}] {}
                                edge from parent
                                node[above] {$yes$}
                            }
                            child [level distance=10em, sibling angle=30]
                            {
                                node[q] {Prompt: Is MIME type known?}
                                    [clockwise from=10]
                                    child [level distance=8em, sibling angle=0]
                                    {
                                        node[end, label=right: {
                                    Prompt with notice of the document type
                                (e.g. ``PDF")\theo{350.295.642}}] {}
                                        edge from parent
                                        node[above] {$yes$}
                                    }
                                    child [level distance=8em, sibling angle=20]
                                    {
                                        node[end, label=right:
                                        {Promt showing MIME type}] {}
                                        edge from parent
                                        node[above] {$no$}
                                    }
                                edge from parent
                                node[above] {$no$}
                            }
                        edge from parent
                        node[above] {$no$}
                    }
                edge from parent
                node[above] {$yes$}
            }
            child [level distance=8em, sibling angle=100]
            {
                node[q] {Sniff. Is auto-open set?}
                    [clockwise from=10]
                    child [level distance=8em, sibling angle=0]
                    {
                        node[end, label=right: {
                            Auto open
                        }] {}
                        edge from parent
                        node[above] {$yes$}
                    }
                    child [level distance=6em, sibling angle=15]
                    {
                        node[end, label=right:
                        {?}] {}
                        node[above] {$no$}
                    }
                edge from parent
                    node[below] {$no$}
            }
        edge from parent
            node[below] {$no$}
    }
    ;
\end{tikzpicture}
\caption{Firefox auto-download settings}
\end{figure*}

\subsubsection{Browser: Opera}
\label{subsubsec:opera_mime_handling}

\begin{figure*}
    \centering
    \includegraphics[width=0.95\textwidth]{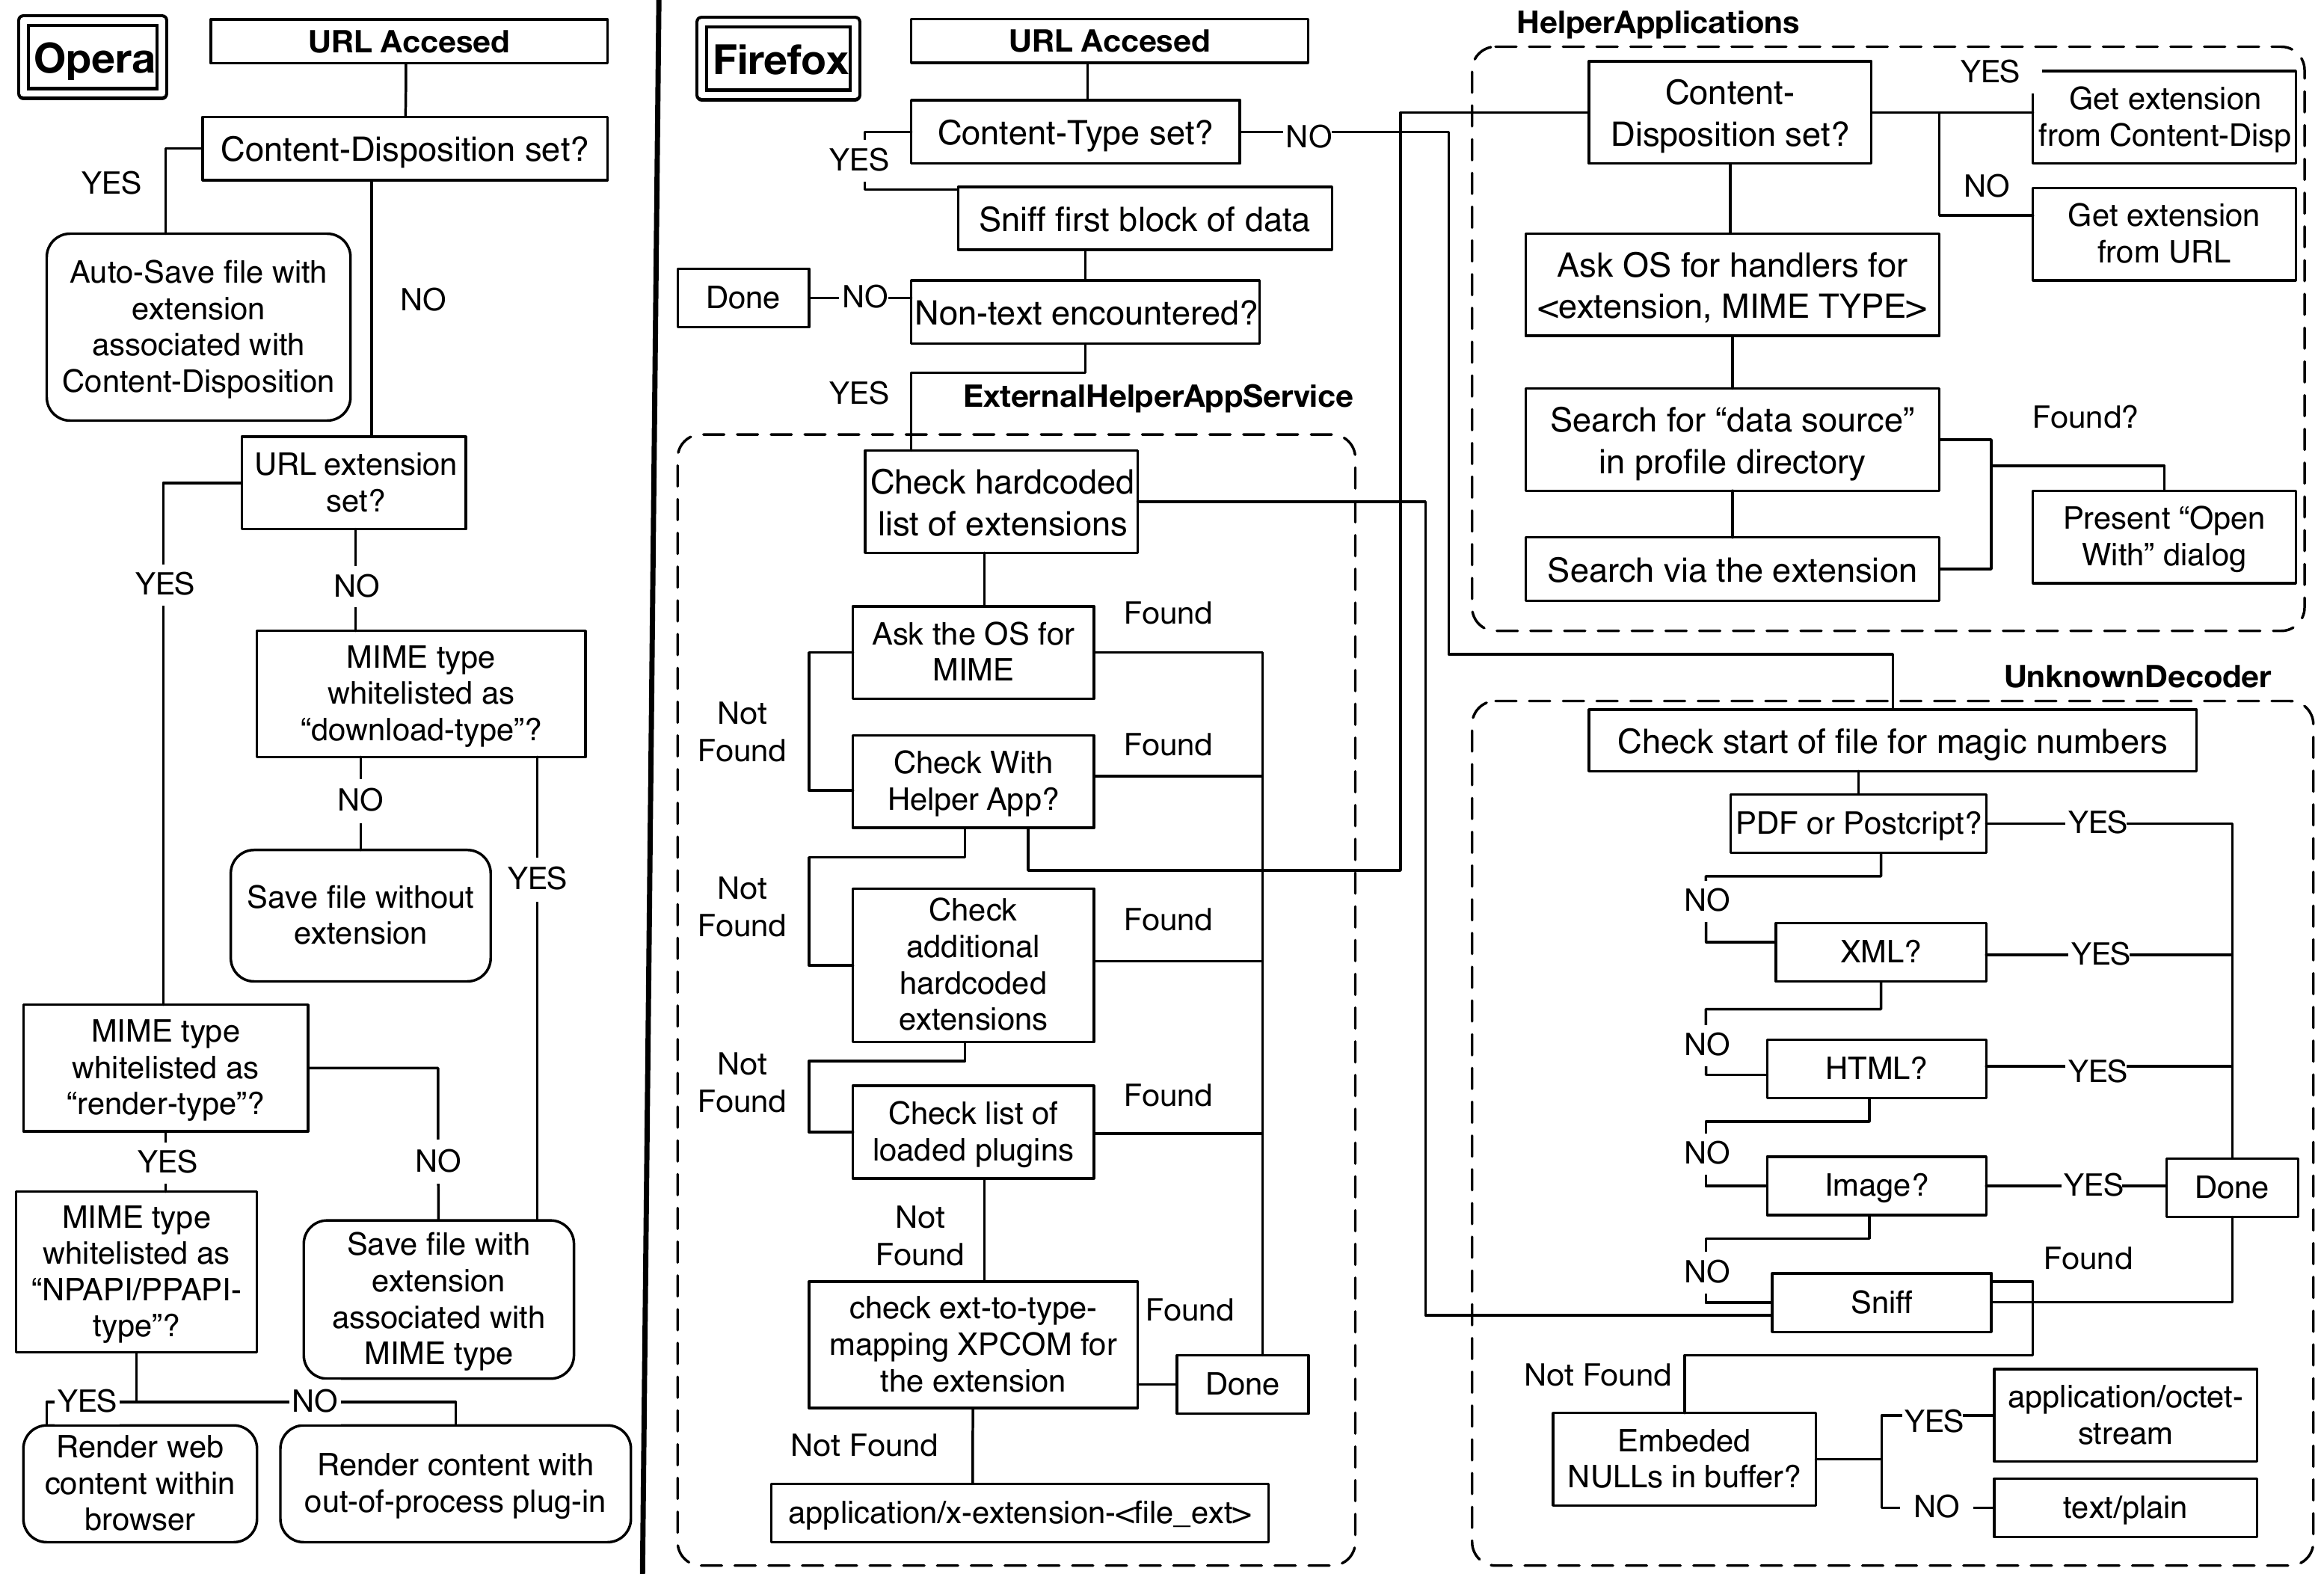}
    \caption{Display/download behavior of Opera.}
    \label{fig:opera_behavior}
\end{figure*}

\subsubsection{Browser: Safari}
\label{subsubsec:safari_mime_handling}

\subsection{Mobile Browser MIME-Type Handling}
\label{subsection:mobile_br_handling}

\subsubsection{Chrome (Android)}
\label{subsubsec:chrome_andr_mime_handling}
\textit{Rendering}

\subsubsection{Safari (iOS)}
\label{subsubsec:safari_ios_mime_handling}
\textit{Rendering}

\subsection{Automatic actions and extended file attributes}
\label{subsec:auto}

\subsubsection{Linux}
\label{subsubsec:auto_linux}
Modern ext filesystems used in Linux support file extended attributes, however
this option must be enabled in the kernel config.
Attributes can be read and set using the \texttt{setfattr} and \texttt{getfattr}
commands which are part of the \texttt{attr} package, as well as the
\texttt{xattr} command which are part or the \texttt{python-xattr}.
Respectively, attributes are changed using the \texttt{chattr} command.

Currently on Linux there are four namespaces for extended file attributes,
namely \texttt{user, trusted, security} and \texttt{system}.  The
\texttt{system} namespace
is used primarily by the kernel for access control lists (ACLs) and can only be
set by root. For example, it will use names such as
\texttt{system.posix\_acl\_access}
and \texttt{system.posix\_acl\_default} for extended file attributes. The
\texttt{security} namespace is used by SELinux~\cite{selinux}

Whenever a file gets downloaded by the internet, its origin url is stored in the
dedicated extended attribute \texttt{user.xdg.origin.url}. If there was a
referrer URL present, the respective attribute is also set in
\texttt{user.xdg.referrer.url}

\theo{Discussion on auto-download per browser, permissions after download in the
OS as well as file quarantine information}

\textit{X Permissions}: After downloading a simple executable file
(using either Chrome or Mozilla),
the permissions are the following: {\tt -rw-rw-r--}.
Hence, the user cannot execute it.
Nevertheless, if the file is compressed (.zip),
then the user can execute is right away ({\tt -rwxrwxr-x}).

\subsubsection{Mac OS X}
\label{subsubsec:auto_mac}
\textbf{xattr}: Extended attributes for various files can be listed via
\texttt{xattr -l}.
\begin{itemize}
    \item \texttt{com.apple.FinderInfo} contains information for
        Finder.app (\eg folder colors)
    \item \texttt{com.apple.metadata} contains Spotlight data (\eg, download
        location, version info, origin URL)
    \item \texttt{com.apple.quarantine} attribute is set by
        \textit{quarantine-aware} applications
\end{itemize}

Essentially, the URL from which a file is downloaded, as well as the application
that downlloaded the file, a unique ID and a timestamp is stored in a sqlite3
DB, which can be read via
\texttt{\tiny{sqlite3
~/Library/Preferences/com.apple.LaunchServices.QuarantineEventsV2}}

If an application has the \texttt{Info.plist} key
\texttt{LSFileQuarantineEnabled} set, all files created by that application will
be quarantined by OS X

The process in which the OS handles quarantined files can depicted in
Fig.~\ref{fig:mac_gatekeeper}

\textit{X Permissions}: After downloading a simple executable file
(using either Chrome, Mozilla or Safari),
the permissions are the following: {\tt -rw-r--r--}.
Hence, the user cannot execute it.
Note that,
contrary to Mac OS X the permissions of the members change here
(read-only).
However, just like in Linux, if the file is compressed,
the file is executable ({\tt -rwxr-xr-x}).

\subsubsection{Windows}

\textit{X Permissions}: After downloading a simple executable
(.bat) file using either Chrome, Mozilla or IE,
the user can execute it right away (IE explorer warns the
user though).

\begin{figure}[!h]
    \centering
    \includegraphics[width=0.85\columnwidth]{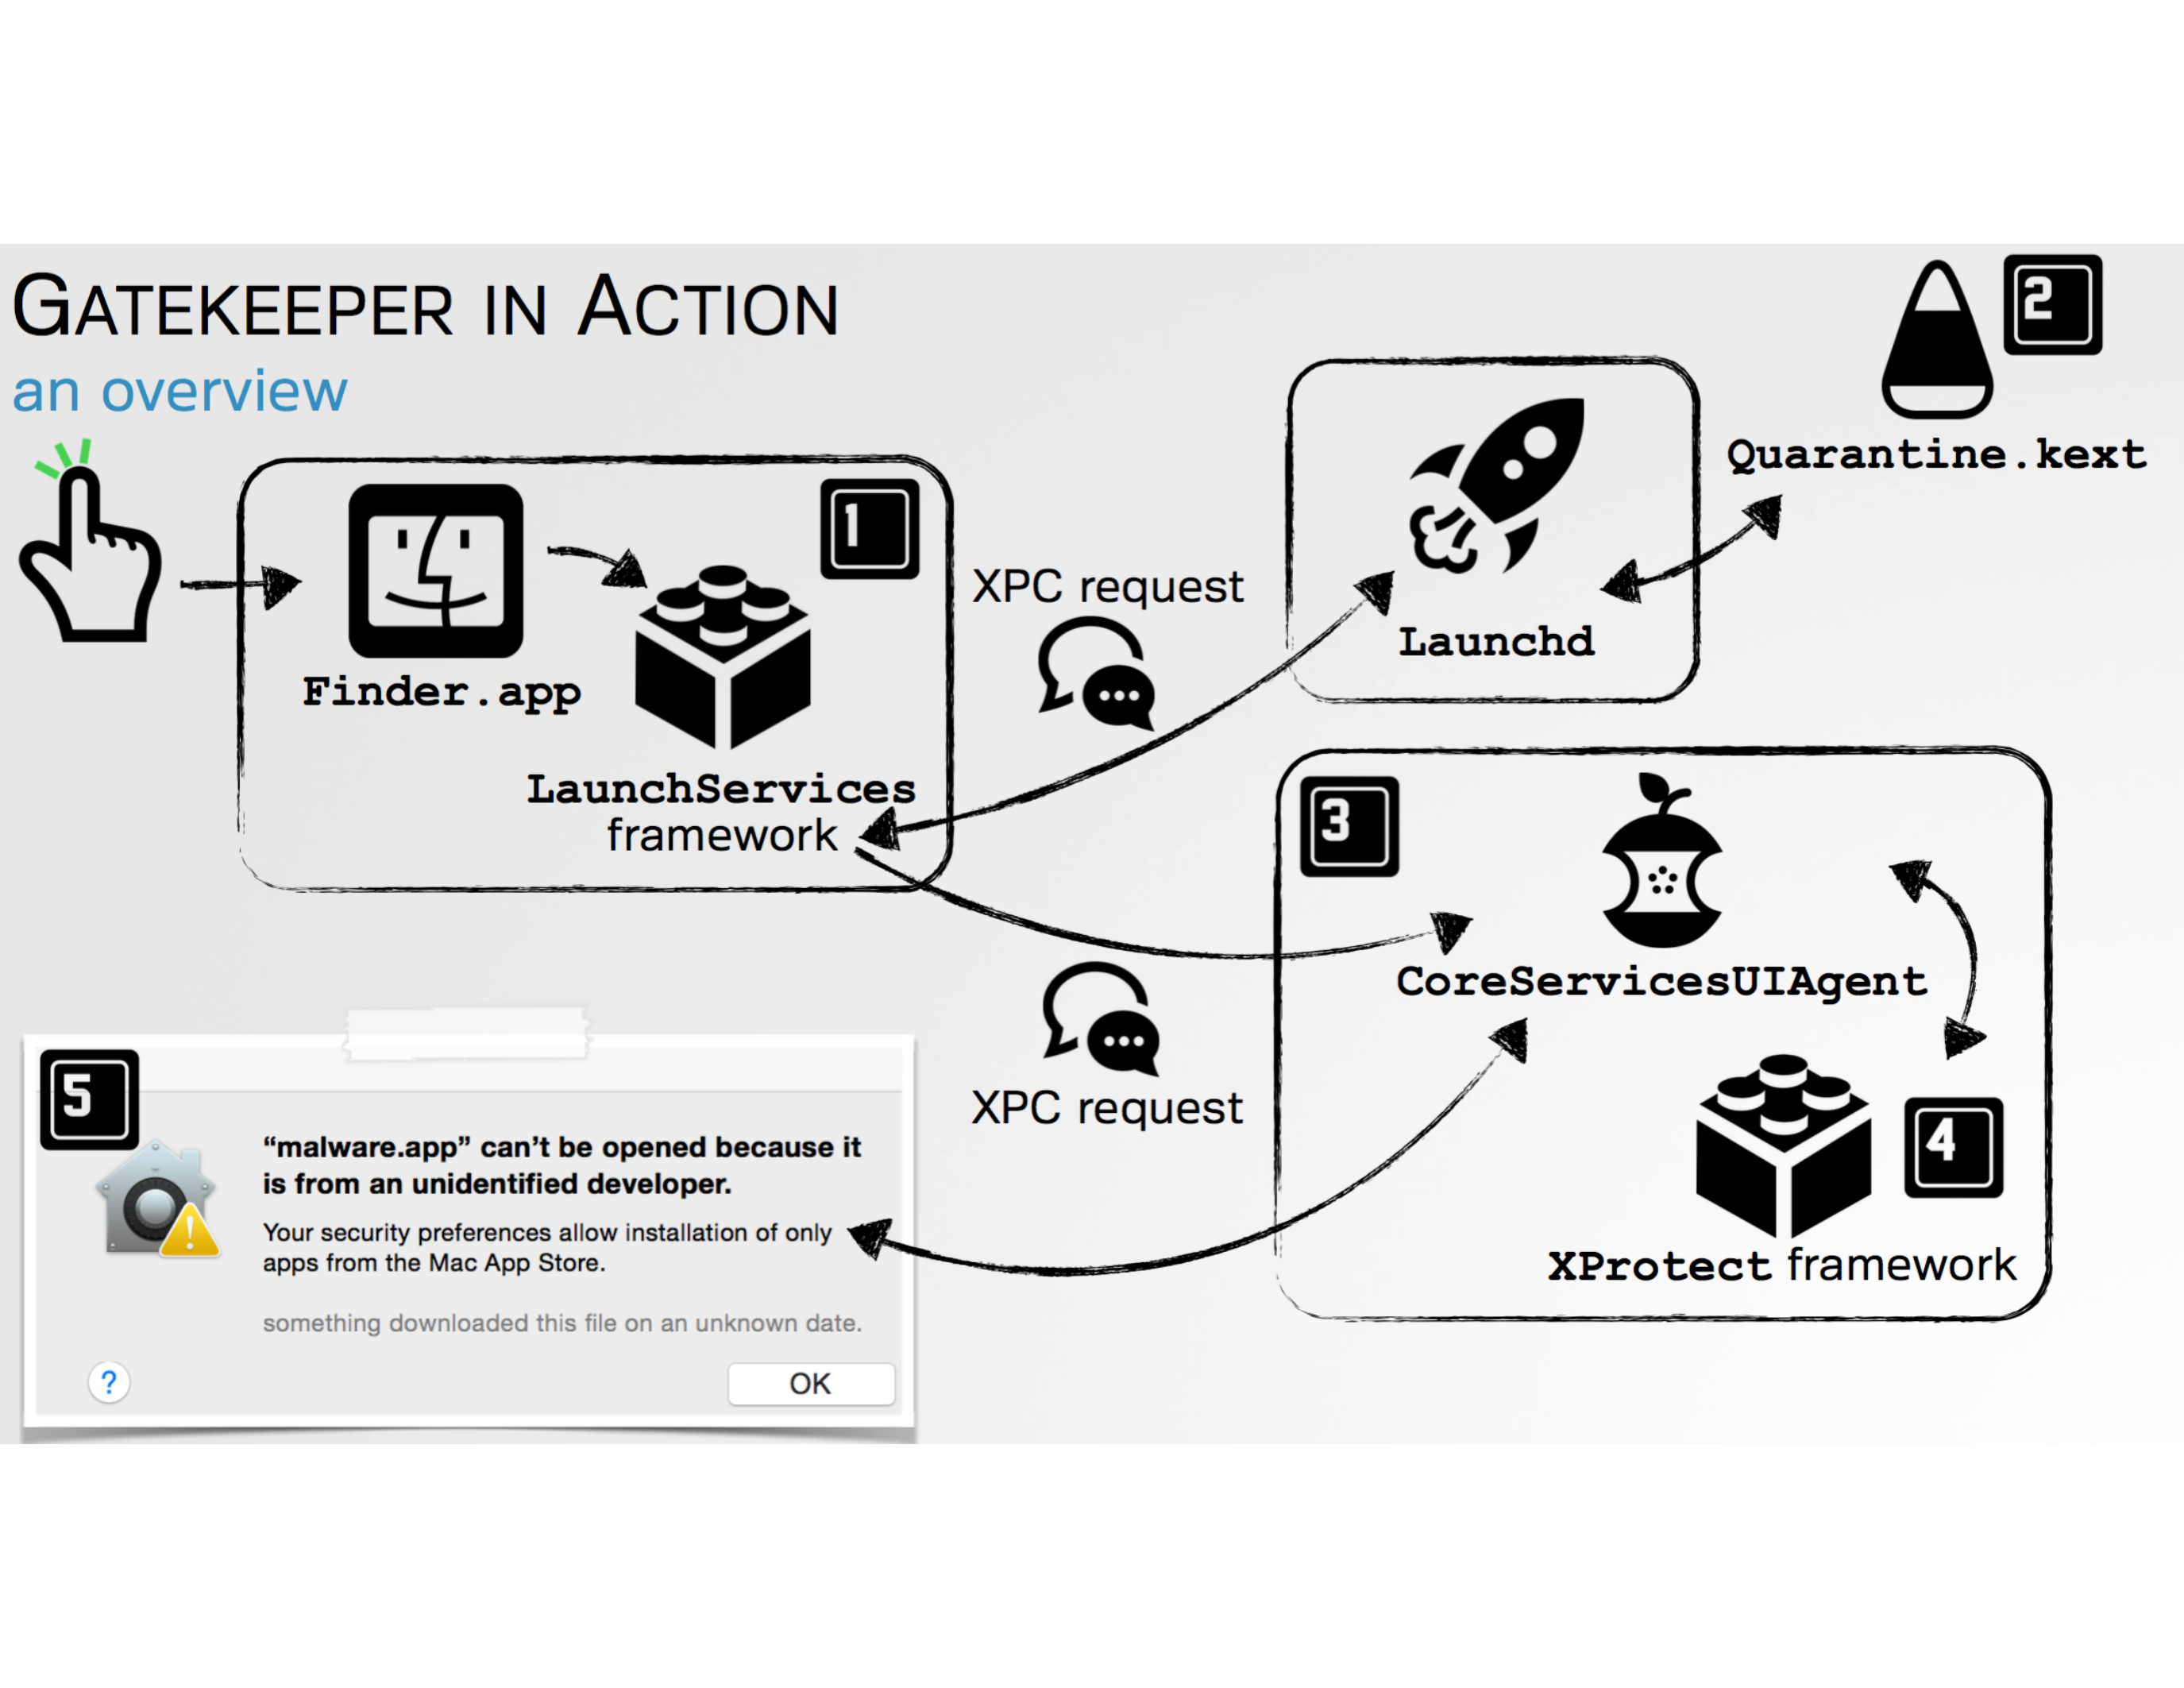}
    \caption{Gatekeeper}
    \label{fig:mac_gatekeeper}
\end{figure}

\afterpage{\clearpage}
\subsection{Known Attacks}
\label{subsec:known_attacks}

\subsubsection{CSS Cross-Origin Attacks}
\label{subsubsec:css_attacks}
Cascading Style Sheet Cross-Origin attacks
Such attacks have been shown possible due to discrepancies between browsers'
\textit{standard} and \textit{Quircks} modes of parsing Document Type
Definitions (DTDs)~\cite{Keith:online}.

\subsubsection{XSS Attacks}
\label{subsubsec:xss_attacks}

XSS exploiting Browsers' MIME Sniffing~\cite{mimesniff:online,
MS_MIME:online, Risky47:online} falls withing the more general case of XSS
exploitation using MIME Type Mismatch

\subsubsection{Local Execution Attacks}
\label{subsubsec:local_exec_attacks}

The security implications of the \textit{auto-open} settings in browsers are not
new~\cite{safari_shell:online}. Malicious files often have fake file
extensions~\cite{fake_file_ext:online} or have no extension at all but employ
unicode character tricks to appear as if a legal extension is
present~\cite{packetstorm_unicode:online}

Privilege escalation attacks due to javascritp vulnerabilities have been shown
capable of allowing loading of local files and browser-specific privileged pages
into an iframe~\cite{CVE-2013-5598:online}
